# Supplementary material for: Proximity Based Load Balancing Policies on Graphs: A Simulation Study
Source: arXiv:2011.01485 source file (2020-11-03)
Supplement: Supplementary file 1 [file appendix.tex]

%%%!TEX PS-program = pdflatexmk
%%!TEX root = POT_sigmetrics21.tex
